# Supplementary material for: Depth Reconstruction with Neural Signed Distance Fields in Structured Light Systems
Source: arXiv:2405.12006 source file (2024-05-20)
Supplement: Supplementary file 1 [file X_suppl.tex]

\clearpage
\setcounter{page}{1}
\maketitlesupplementary

\section{Training settings}
Our framework is implemented using PyTorch learning framework. In each iteration, we randomly select 2048 points for training. For each light ray originating from a camera pixel, a total of 64 points are sampled: 32 for the initial coarse sampling and 32 for subsequent finer sampling. The nearest and farthest boundaries are set to $0.5m$ and $1.0m$, respectively. The camera captures the images at a resolution of $1280\times1024$, while the projector projects patterns at $1280\times800$. % We use a bounding box to speed up the training and avoid meaningless sampling. The bounding box is computed based on the maximum and minimum value of captured images, 

\begin{figure}
    \centering
    \includegraphics[width=1.0\linewidth]{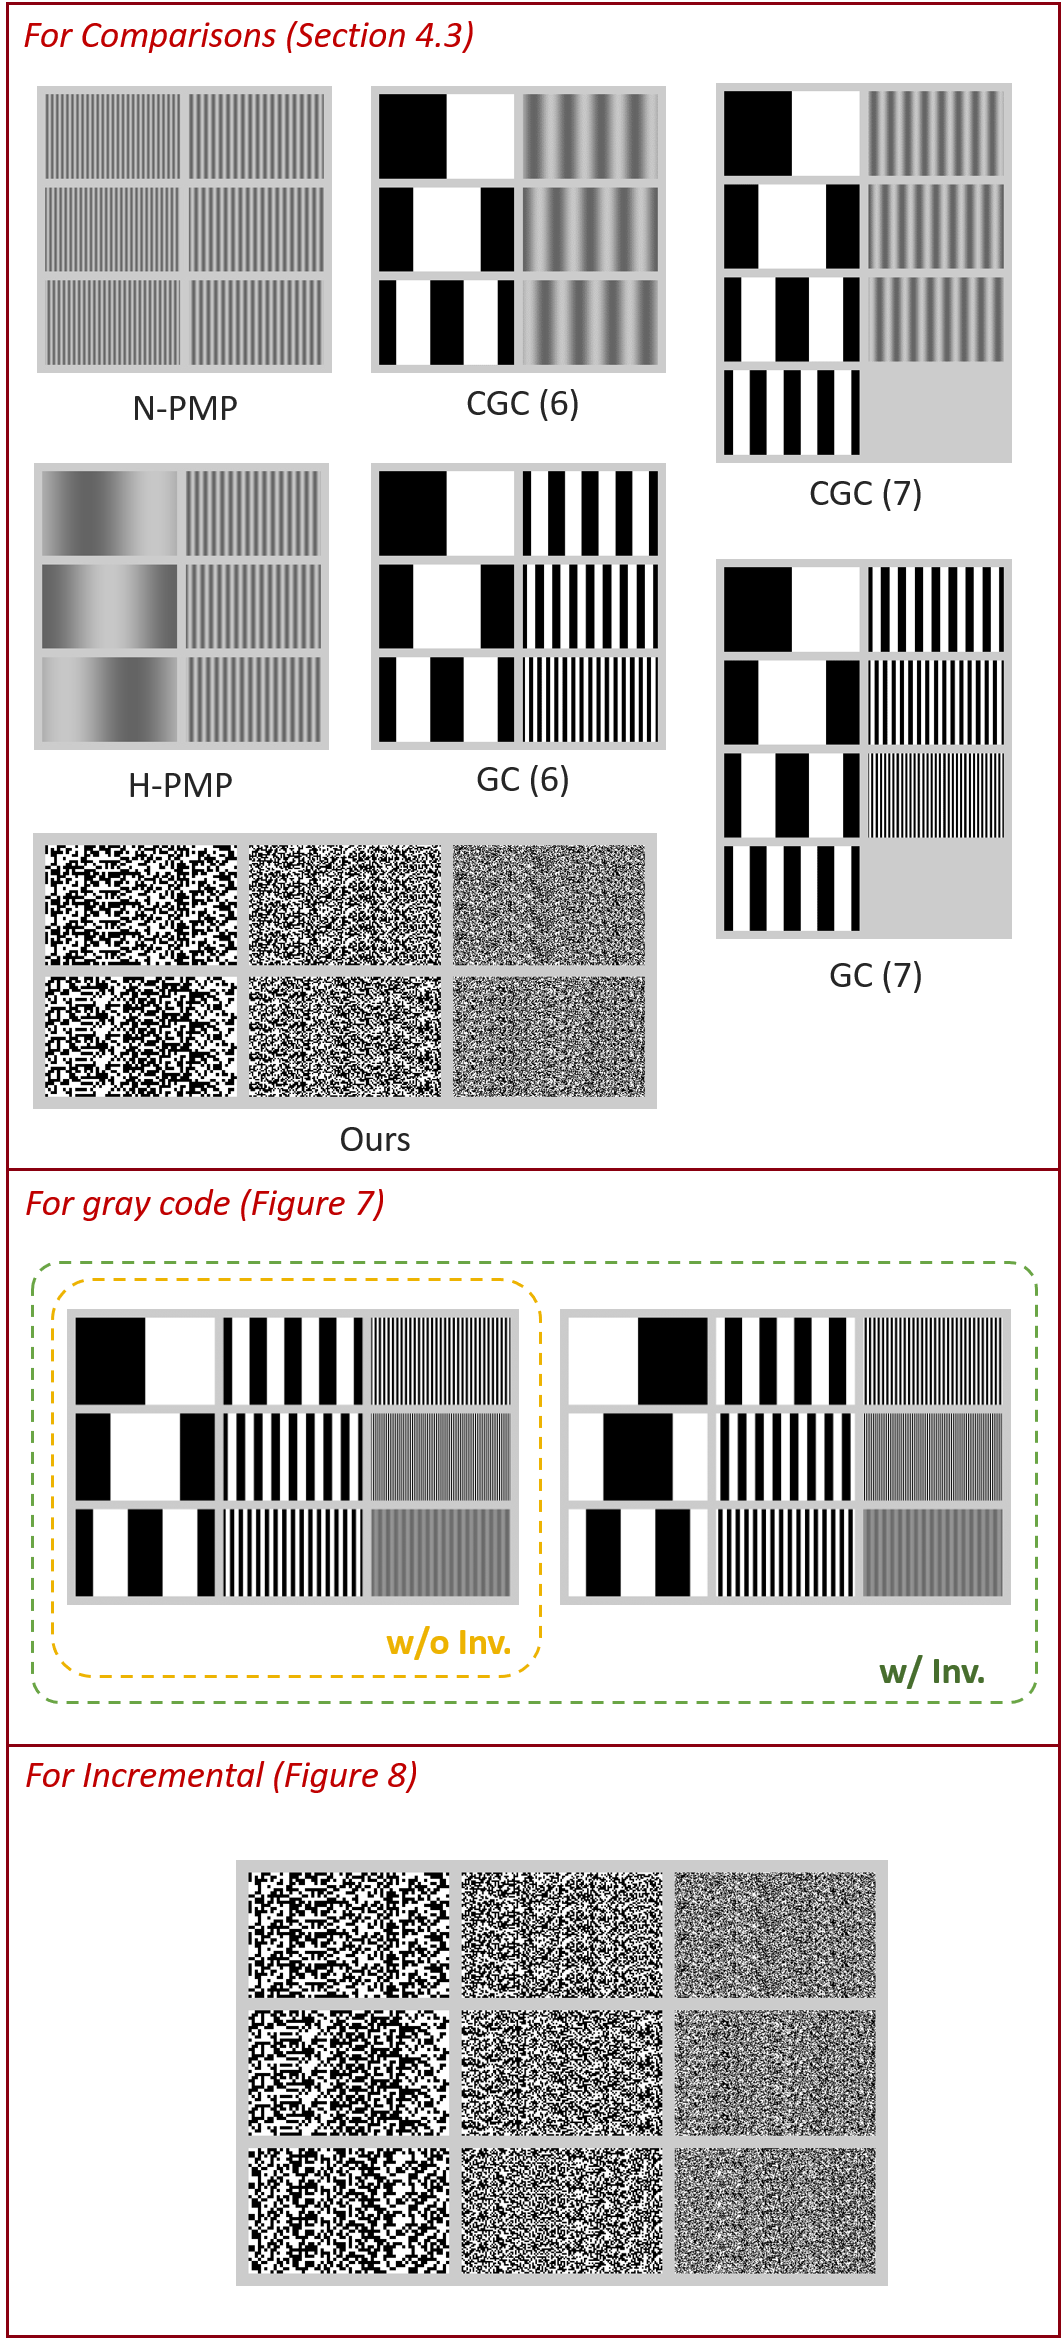}
    \caption{Patterns used for each experiments.}
    \label{fig:patternsup}
\end{figure}

% \begin{figure}
%     \centering
%     \includegraphics[width=\linewidth]{3DV-First/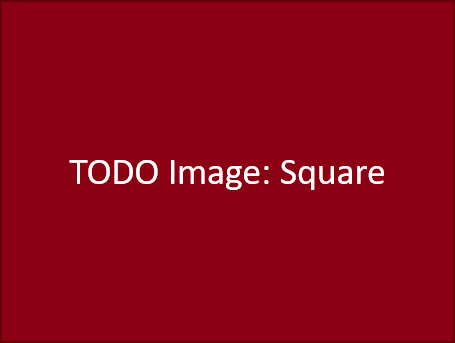}
%     \caption{Patterns used for each experiments.}
%     % \label{fig:patternsup}
% \end{figure}

\section{Patterns for experiments}
As depicted in \Cref{sec:patterndesign}, the unit square is randomly assigned black or white. We generate a pattern with a resolution of $1280\times200$, repeating it vertically 4 times due to our device's horizontal placement. In practice, we observed the projector encountering scatter issues, causing blurry and indistinct projected patterns. In this context, the minimum recognizable length is approximately 5 pixels, influencing our pattern setting where 5 pixels constitute the minimum unit length. All pattern sets utilized for the experiments are showcased in \cref{fig:patternsup}. 

% 1. Gray Code 对比的数据
\section{Additional experimental results}

We append the quantitative experimental results for gray code comparison and incremental comparison in \Cref{tab:graycodesup} and \Cref{tab:onlinesup}, respectively. For additional visualization results, we kindly refer readers to our attached video for more comprehensive insights.

\begin{table*}
    \begin{center}
        \begin{tabular}{@{}ccccccccccccc@{}}
            \hline
            \multirow{2}*{Num.} & \multicolumn{2}{c}{Scene 1} & \multicolumn{2}{c}{Scene 2} & \multicolumn{2}{c}{Scene 3} & \multicolumn{2}{c}{Scene 4} & \multicolumn{2}{c}{Scene 5} & \multicolumn{2}{c}{Scene 6}\\
            ~ & GC & Ours & GC & Ours & GC & Ours & GC & Ours & GC & Ours & GC & Ours \\
            \hline
            3 & 39.779 & 44.209 & 27.760 & 43.653 & 140.035 & 69.530 & 25.784 & 41.824 & 42.796 & 34.657 & 36.758 & 43.985 \\
            4 & 22.333 & 15.552 & 16.469 & 15.312 & 11.841 & 11.825 & 19.450 & 11.805 & 39.876 & 18.308 & 30.257 & 13.745 \\
            5 & 20.528 & 7.839 & 19.843 & 8.180 & 6.779 & 3.919 & 18.052 & 5.087 & 24.498 & 12.351 & 19.860 & 6.575 \\
            6 & 15.766 & 5.102 & 10.498 & 5.211 & 6.672 & 2.665 & 9.629 & 3.061 & 16.333 & 5.833 & 10.177 & 3.495 \\
            7 & 8.277 & 3.491 & 7.689 & 3.255 & 6.584 & 2.467 & 5.391 & 2.361 & 10.961 & 3.082 & 7.225 & 2.970 \\
            8 & 5.038 & 2.942 & 4.851 & 2.290 & 6.685 & 2.100 & 4.306 & 1.815 & 9.706 & 2.766 & 7.264 & 2.044 \\
            9 & 5.808 & 3.555 & 4.635 & 2.723 & 5.365 & 2.098 & 3.997 & 1.757 & 7.794 & 2.213 & 5.346 & 1.849 \\
            \hline
            3-Inv. & 21.512 & 26.563 & 11.122 & 24.185 & 17.926 & 15.192 & 8.037 & 25.344 & 15.850 & 15.535 & 14.424 & 22.899 \\
            4-Inv. & 10.288 & 10.304 & 5.200 & 10.056 & 9.373 & 8.496 & 4.191 & 5.413 & 11.801 & 7.423 & 14.757 & 7.665 \\
            5-Inv. & 5.573 & 5.190 & 2.631 & 4.124 & 6.302 & 4.327 & 2.310 & 2.731 & 7.637 & 3.761 & 10.754 & 3.467 \\
            6-Inv. & 4.288 & 3.846 & 1.855 & 3.382 & 4.818 & 2.633 & 1.679 & 2.508 & 5.038 & 3.068 & 5.726 & 2.421 \\
            7-Inv. & 3.088 & 2.438 & 1.639 & 1.921 & 4.027 & 2.629 & 1.540 & 2.220 & 3.798 & 2.381 & 3.333 & 1.782 \\
            8-Inv. & 2.348 & 2.741 & 1.660 & 1.853 & 3.594 & 2.288 & 1.479 & 1.522 & 3.375 & 2.236 & 2.398 & 2.203 \\
            9-Inv. & 2.638 & 2.571 & 1.981 & 1.733 & 3.494 & 2.388 & 1.717 & 1.459 & 3.284 & 2.089 & 2.285 & 2.583 \\
            \hline
        \end{tabular}
    \end{center}
    \caption{Quantitative experimental results for gray code comparison.}
    \label{tab:graycodesup}
\end{table*}

\begin{table*}
    \begin{center}
        \begin{tabular}{@{}ccccccccccccc@{}}
            \hline
            \multirow{2}*{Num.} & \multicolumn{2}{c}{Scene 1} & \multicolumn{2}{c}{Scene 2} & \multicolumn{2}{c}{Scene 3} & \multicolumn{2}{c}{Scene 4} & \multicolumn{2}{c}{Scene 5} & \multicolumn{2}{c}{Scene 6}\\
            ~ & GC & Ours & GC & Ours & GC & Ours & GC & Ours & GC & Ours & GC & Ours \\
            \hline
            3 & 5.293 & 4.475 & 3.154 & 8.968 & 3.472 & 3.692 & 3.233 & 3.559 & 3.625 & 3.748 & 3.139 & 3.611 \\
            4 & 3.481 & 5.175 & 2.755 & 3.033 & 2.885 & 3.859 & 2.411 & 3.28 & 2.946 & 3.07 & 2.357 & 3.468 \\
            5 & 3.803 & 4.623 & 2.995 & 2.593 & 2.349 & 3.135 & 2.244 & 2.668 & 2.646 & 2.701 & 2.447 & 2.653 \\
            6 & 3.834 & 4.887 & 2.46 & 2.717 & 2.956 & 3.147 & 2.239 & 2.769 & 2.616 & 2.607 & 2.469 & 2.41 \\
            7 & 3.72 & 3.802 & 2.569 & 3.168 & 2.565 & 2.73 & 2.34 & 2.22 & 3.403 & 3.118 & 2.376 & 2.237 \\
            8 & 4.344 & 3.846 & 2.901 & 2.987 & 3.609 & 2.91 & 2.675 & 2.951 & 2.976 & 2.901 & 2.342 & 2.343 \\
            9 & 4.318 & 3.876 & 2.412 & 2.569 & 4.681 & 3.091 & 2.463 & 2.906 & 2.612 & 2.99 & 2.483 & 2.52 \\
            \hline
        \end{tabular}
    \end{center}
    \caption{Quantitative experimental results for incremental comparison.}
    \label{tab:onlinesup}
\end{table*}

% - Patterns

% 可以加OnSurfacePrior。scale=10.0。待会再测试一个100的？或者直接这么搞。
